# Supplementary material for: Scale-Equivariant Unrolled Neural Networks for Data-Efficient Accelerated MRI Reconstruction
Source: arXiv:2204.10436 source file (2022-04-21)
Supplement: Supplementary file 1 [file supplementary.tex]

\section*{Supplementary}

\insertmraugmentconfig
\insertreconexamples
\insertequiverror
\insertstepsize
\insertbenchmark
